# Supplementary material for: Hypercontracts
Source: arXiv:2106.02449 source file (2021-10-08)
Supplement: Supplementary file 1 [file hypercontractsAndAgContracts.tex]

Now we express AG contracts using hypercontracts. 
We can
instantiate trace properties as a $\catCmpSet$ lattice. Each \compset is of the
form $\cmpSet = 2^\cmp$ for some component $\cmp \subseteq \behaviorUnv$.
Observe that the satisfaction of a \compset by a component $\cmp' \in 2^{\cmp}$
happens if and only if $\cmp' \le \cmp$. The meet of two \compsets $2^\cmp \meet
2^{\cmp'}$ is $2^{\cmp \setint \cmp'} = 2^{\cmp} \setint 2^{\cmp'}$, but the
join of two elements $2^\cmp \vee 2^{\cmp'}$ is $2^{\cmp \setunion \cmp'} \ne
2^\cmp \setunion 2^{\cmp'}$. The composition of two \compsets is given by
$2^{\cmp} \times 2^{\cmp'} = 2^{\cmp \setint \cmp'}$, and the quotient is
$2^{\cmp} / 2^{\cmp'} = 2^{\cmp / \cmp'}$.

Assume-guarantee contracts are often given as a
pair of trace-properties $(A, G)$, where $A$ states the assumptions made on the
environment, and $G$ states what the component in question should guarantee when
operating in a valid environment (i.e., one that meets the assumptions). We
observe that any closed system obtained using environments that meet the
assumptions is restricted to $G \setint A$; thus, we set the closed-system spec
to $\sysSet = 2^{A \setint G}$. Define the hypercontract $\cont = (2^A, 2^{A
\setint G})$. The environments are $\envSet = 2^A$, namely, all $E \subseteq A$,
and the implementations are $\impSet = 2^{(A \setint G)/A} = 2^{G / A}$, that
is, all $\cmp \subseteq G / A$. Observe that $\sysSet / \impSet = \envSet$, so
$\cont$ is saturated. Now suppose we have another hypercontract $\cont' =
(2^{A'}, 2^{A' \setint G'})$ with environments $\envSet'$ and implementations
$\impSet'$. We observe that $\envSet \le \envSet'$ if and only if $A \subseteq
A'$; moreover, $\impSet' \le \impSet$ if and only if $G' / A' \le G / A$. This
means that $\cont' \le \cont$ if and only if the assume-guarantee contracts $(A,
G)$ and $(A', G')$ satisfy $(A', G') \le (A, G)$.

Suppose we
have a second hypercontract $\cont' = (2^{A'}, 2^{G' / A'})$. Applying
\eqref{eq:cntComp}, we obtain a composition formula for these hypercontracts:
$\cont \contComposition \cont' = \left( 2^{A' / (G / A)} \right. \meet \linebreak[1] \left. 2^{A/(G'/A')},
2^{G/A} \meet 2^{G'/A'} \right)$, whose environments and implementations are
exactly those obtained from the composition of the assume-guarantee contracts
$(A, G)$ and $(A', G')$ \cite{Benveniste2008}.

Given two assume-guarantee contracts $(A_i, G_i)$
for $i = 1,2$, we consider the merging of their hypercontracts. We have
$(2^{A_1}, 2^{A_1 \setint G_1}) \bullet (2^{A_2}, 2^{A_2 \setint G_2}) = (2^{A_1
\setint A_2}, 2^{A_1 \setint G_1 \setint A_2 \setint G_2})$. Observe that this
last hypercontract has environments $2^{A_1 \setint A_2}$ and implementations
$2^{(G_1 \setint G_2) / (A_1 \setint A_2)}$. This is the definition of merging
for assume-guarantee contracts \cite{agContractMerging}.

%Appendix \ref{xknskaJK} shows a novel extension of AG contracts in which
%environments and implementations are allowed to state not only allowed
%behaviors, but also required behaviors, in the style of modal interfaces.
