# Supplementary material for: Hypercontracts
Source: arXiv:2106.02449 source file (2021-10-08)
Supplement: Supplementary file 2 [file additionalReceptiveProofs.tex]

%\begin{proof}[Proof of Proposition \ref{hbaixoib}]
    \begin{proof}[Proof of Proposition 5.7]
    
\end{proof}
