# Supplementary material for: Hypercontracts
Source: arXiv:2106.02449 source file (2021-10-08)
Supplement: Supplementary file 3 [file EMSOFT21_AdditionalProofs.pdf]

# Hypercontracts

ANONYMOUS AUTHOR(S)

Contracts (or interface) theories have been proposed to formally support distributed and decentralized system design while ensuring safe system integration. Over the last decades, a number of formalisms were proposed, sometimes very different in their form and algebra. This motivated the quest for a unification by some authors, e.g., specifications through contracts by Bauer et al. and the contract metatheory by Benveniste et al. to cite a few. These generic models establish precise links between the different contract frameworks. In this paper we propose *hypercontracts*, a generic model with a richer structure for its underlying model of components, subsuming simulation preorders. While this new model remains generic, it provides a much more elegant and richer algebra for its key notions of refinement, parallel composition, and quotient, and it allows considering new operations. On top of these foundations, we propose *conic hypercontracts*, which are still generic but come with a finite description. We show how to specialize conic hypercontracts to Assume-Guarantee contracts as well as to Interface Automata, two known contract frameworks very different in style. We illustrate conic hypercontracts on specifications involving security and the robustness of machine-learning components.

CCS Concepts: • **Computer systems organization** → **Embedded and cyber-physical systems; Embedded and cyber-physical systems**; • **Theory of computation** → **Formalisms; Formalisms**; • **Computing methodologies** → **Modeling methodologies**.

Additional Key Words and Phrases: contracts, hypercontracts, contract-based design, component-based design, assume-guarantee, hyperproperties, downward-closed

## ACM Reference Format:

Anonymous Author(s). 2021. Hypercontracts. *ACM Trans. Embedd. Comput. Syst.* x, x, Article x (August 2021), 4 pages. <https://doi.org/10.1145/1122445.1122456>

## B PROOFS OF ADDITIONAL CLAIMS

PROOF OF PROPOSITION 5.7. From the principle of hypercontract composition, we must have

$$E_R \leq U \stackrel{\text{def}}{=} (E_{S'}/M_S) \wedge (E_S/M_{S'}) \text{ and} \quad (17)$$

$$L \stackrel{\text{def}}{=} M_{S'} \times M_S \leq M_R. \quad (18)$$

Observe that the quotients  $E_{S'}/M_S$  and  $E_S/M_{S'}$  both have io signature  $O \cup O'$ , so the conjunction in (17) is well-defined as an operation of the Heyting algebra  $\mathcal{L}_{O \cup O'}$ . We study the first element:

$$E_{S'}/M_S = (E_{S'} \cap M_S \cup \text{MissExt}(E_{S'}, M_S, O)) \setminus \text{Unc}(E_{S'}, M_S, O, O').$$

We attempt to simplify the terms. Suppose  $w \in E_{S'} \cap (M_S \setminus S)$ . Then all extensions of  $w$  lie in  $M_S \setminus S$ . This means that  $\text{MissExt}(E_{S'}, M_S, O) = \text{MissExt}(E_{S'}, S, O)$ . Moreover, if a word is an element of  $E_{S'} \setminus S'$ , all its extensions are in this set, as well (i.e., it is impossible to escape this set by extending words). Thus,  $\text{Unc}(E_{S'}, M_S, O, O') = \text{Unc}(S', M_S, O, O')$ . We have

$$E_{S'}/M_S = (E_{S'} \cap M_S \cup \text{MissExt}(E_{S'}, S, O)) \setminus \text{Unc}(S', M_S, O, O').$$

---

Permission to make digital or hard copies of all or part of this work for personal or classroom use is granted without fee provided that copies are not made or distributed for profit or commercial advantage and that copies bear this notice and the full citation on the first page. Copyrights for components of this work owned by others than ACM must be honored. Abstracting with credit is permitted. To copy otherwise, or republish, to post on servers or to redistribute to lists, requires prior specific permission and/or a fee. Request permissions from [permissions@acm.org](mailto:permissions@acm.org).

© 2021 Association for Computing Machinery.

1539-9087/2021/8-ARTx \$15.00

<https://doi.org/10.1145/1122445.1122456>

Now we can write

$$U = [(E_{S'} \cap M_S \cup \text{MissExt}(E_{S'}, S, O)) \cap (E_S \cap M_{S'} \cup \text{MissExt}(E_S, S', O'))] \setminus [\text{Unc}(S', M_S, O, O') \cup \text{Unc}(S, M_{S'}, O', O)].$$

Observe that

$$\begin{aligned} E_{S'} \cap M_S \cap \text{MissExt}(E_S, S', O') &= (S' \cup \text{MissExt}(S', S', O')) \cap M_S \cap \text{MissExt}(E_S, S', O') \\ &= M_S \cap \text{MissExt}(E_S, S', O') = M_S \cap \text{MissExt}(S, S', O'). \end{aligned}$$

The last equality comes from the following fact: if a word of  $\text{MissExt}(E_S, S', O')$  is obtained by extending a word of  $(E_S \setminus S) \cap S'$  by  $O'$ , the resulting word is still an element of  $E_S$ , which means it cannot be an element of  $M_S$  because  $M_S$  and  $E_S$  are disjoint outside of  $S$ . Therefore,

$$U = \left[ \begin{array}{l} (S \cap S') \cup \\ (M_S \cap \text{MissExt}(S, S', O')) \cup \\ (M_{S'} \cap \text{MissExt}(S', S, O)) \cup \\ (\text{MissExt}(E_{S'}, S, O) \cap \text{MissExt}(E_S, S', O')) \end{array} \right] \setminus [\text{Unc}(S', M_S, O, O') \cup \text{Unc}(S, M_{S'}, O', O)]. \quad (19)$$

We can write

$$\begin{aligned} \text{MissExt}(E_{S'}, S, O) \cap \text{MissExt}(E_S, S', O') &= \\ &\text{MissExt}(E_{S'}, S, O) \cap \text{MissExt}(S, S', O') \cup \\ &\text{MissExt}(S', S, O) \cap \text{MissExt}(E_S, S', O') \cup \\ &\text{MissExt}(\text{MissExt}(S', S', O'), S, O) \cap \text{MissExt}(\text{MissExt}(S, S, O), S', O'). \end{aligned}$$

Note that  $\text{MissExt}(E_{S'}, S, O) \cap \text{MissExt}(S, S', O') = \text{MissExt}(S, S, O) \cap \text{MissExt}(S, S', O')$ . Hence

$$\begin{aligned} & (M_S \cap \text{MissExt}(S, S', O')) \cup (\text{MissExt}(E_{S'}, S, O) \cap \text{MissExt}(S, S', O')) \\ &= \text{MissExt}(S, S', O') \cap (M_S \cup \text{MissExt}(E_{S'}, S, O)) \\ &= \text{MissExt}(S, S', O') \cap (M_S \cup \text{MissExt}(S, S, O)) = \text{MissExt}(S, S', O'). \end{aligned}$$

Finally, we observe that the set  $\text{MissExt}(\text{MissExt}(S', S', O'), S, O) \cap \text{MissExt}(\text{MissExt}(S, S, O), S', O')$  must be empty since the words of the first term have prefixes in  $S \setminus S'$ , and the second in  $S' \setminus S$ . These considerations allow us to conclude that

$$U \leq \left[ \begin{array}{l} (S \cap S') \cup \\ \text{MissExt}(S, S', O') \cup \\ \text{MissExt}(S', S, O). \end{array} \right] \setminus [\text{Unc}(S', M_S, O, O') \cup \text{Unc}(S, M_{S'}, O', O)].$$

To simplify the expression a step further, suppose  $w \in \text{Unc}(S', M_S, O, O')$  and has a prefix in  $S' \cap (M_S \setminus S)$ . Then  $w \notin S \cap S'$ . The words of  $\text{MissExt}(S, S', O')$  do not have prefixes in  $S' \setminus S$ , so  $w \notin \text{MissExt}(S, S', O')$ . The words of  $\text{MissExt}(S', S, O)$  belong to  $E_S$ , which is disjoint from  $M_S$  outside of  $S$ . Thus,  $w \notin \text{MissExt}(S', S, O)$ .

We just learned that the words of  $\text{Unc}(S', M_S, O, O')$  having a prefix in  $S' \cap (M_S \setminus S)$  are irrelevant for the inequality above. Now consider a word  $w$  of  $\text{Unc}(S', M_S, O, O')$  with no prefix in  $S' \cap (M_S \setminus S)$ . Let  $w_p$  be the longest prefix of  $w$  which is in  $S \cap S'$ . There is a word  $w' \in (O \cup O')^*$  and a symbol  $\sigma \in O$  such that  $w_p \circ w' \in S' \cap M_S$  and  $w_p \circ w' \circ \sigma \in M_S \setminus S'$ . Suppose  $w'$  is not the empty string. Then we can let  $\sigma'$  be the first symbol of  $w'$ . Then  $w_p \circ \sigma' \in M_S \setminus S$ , so  $\sigma' \in O'$ . But this means that  $w \in \text{Unc}(S, S', O', O)$ . If  $w'$  is empty,  $w_p \in S \cap S'$  and  $w_p \circ \sigma' \in M_S \setminus S'$ . Since  $\sigma \in O$ ,  $w_p \circ \sigma \in \cap M_S$

if and only if it belongs to  $S$ . Thus,  $w_p \circ \sigma' \in S \setminus S'$ , which means that  $w \in \text{Unc}(S', S, O, O')$ . We can thus simplify the upper bound on  $E_R$  to

$$U = \left[ \begin{array}{c} (S \cap S') \cup \\ \text{MissExt}(S, S', O') \cup \\ \text{MissExt}(S', S, O) \end{array} \right] \setminus [\text{Unc}(S', S, O, O') \cup \text{Unc}(S, S', O', O)]. \quad (20)$$

Define  $\hat{R} \stackrel{\text{def}}{=} (S \cap S') \setminus [\text{Unc}(S', S, O, O') \cup \text{Unc}(S, S', O', O)]$ . We want to show that  $U = \hat{R} \cup \text{MissExt}(\hat{R}, \hat{R}, O \cup O')$ . Note that we only have to prove that

$$\text{MissExt}(\hat{R}, \hat{R}, O \cup O') = \left[ \begin{array}{c} \text{MissExt}(S, S', O') \cup \\ \text{MissExt}(S', S, O) \end{array} \right] \setminus [\text{Unc}(S', S, O, O') \cup \text{Unc}(S, S', O', O)]. \quad (21)$$

PROOF OF (21). Suppose  $w \in \text{MissExt}(S, S', O') \setminus [\text{Unc}(S', S, O, O') \cup \text{Unc}(S, S', O', O)]$ . Write  $w = w_p \circ \sigma \circ w'$ , where  $w_p$  is the longest prefix of  $w$  which lies in  $S \cap S'$ ,  $\sigma \in O'$ , and  $w' \in \Sigma^*$ .  $w_p \notin [\text{Unc}(S', S, O, O') \cup \text{Unc}(S, S', O', O)]$  because all its extensions would be in this set if  $w_p$  were in this set, and we know that  $w$  is not in this set. It follows that  $w_p \in \hat{R}$  and since  $w_p \circ \sigma \notin \hat{R}$ ,  $w_p \circ \sigma$  and all its extensions are in  $\hat{R} \cup \text{MissExt}(\hat{R}, \hat{R}, O \cup O')$ . Thus,  $w \in \hat{R} \cup \text{MissExt}(\hat{R}, \hat{R}, O \cup O')$ . The same argument applies when

$$w \in \text{MissExt}(S', S, O) \setminus [\text{Unc}(S', S, O, O') \cup \text{Unc}(S, S', O', O)].$$

We conclude that the right hand side of (21) is a subset of the left hand side.

Now suppose that  $w \in \text{MissExt}(\hat{R}, \hat{R}, O \cup O')$  and write  $w = w_p \circ \sigma \circ w'$ , where  $w_p$  is the longest prefix of  $w$  contained in  $\hat{R}$ ,  $\sigma \in O \cup O'$ , and  $w' \in \Sigma^*$ . From the definition of  $\hat{R}$ ,  $w_p \in S \cap S'$ . Suppose  $w_p \circ \sigma \in S \cap S'$ . Then

$$w_p \circ \sigma \in [\text{Unc}(S', S, O, O') \cup \text{Unc}(S, S', O', O)],$$

which means that  $w_p$  also belongs to this set (because  $\sigma \in O \cup O'$ ). This contradicts the fact that  $w_p \in \hat{R}$ , so our assumption that  $w_p \circ \sigma \in S \cap S'$  is wrong. Then  $w_p$  is also the longest prefix of  $w$  contained in  $S \cap S'$ .

Without loss of generality, assume  $\sigma \in O$ . Suppose  $w_p \circ \sigma \notin S$ . Then  $w \in \text{MissExt}(S', S, O)$ . Moreover, since  $w_p \in \hat{R}$ ,  $w_p \circ \sigma \notin [\text{Unc}(S', S, O, O') \cup \text{Unc}(S, S', O', O)]$ . Since  $w_p \circ \sigma \notin S \cap S'$ , we have  $w \notin [\text{Unc}(S', S, O, O') \cup \text{Unc}(S, S', O', O)]$ . Thus,  $w$  is in the right hand set of (21).

Now suppose  $w_p \circ \sigma \notin S'$ . If  $w_p \circ \sigma \in S$ , then  $w_p \in \text{Unc}(S', S, O, O')$ , which contradicts the fact that  $w_p \in \hat{R}$ . We must have  $w_p \circ \sigma \notin S$ , which we already showed implies that  $w$  is in the right hand set of (21).

An analogous reasoning applies to  $\sigma \in O'$ . We conclude that the right hand side of (21) is a subset of the left hand side, and this finishes the proof of their equality. ■

This result and (17) tell us that  $E_R \leq \hat{R} \cup \text{MissExt}(\hat{R}, \hat{R}, O \cup O')$ . Now we study the constraint (18). We want to show that  $\hat{R}$  yields the tightest bound  $L \leq \hat{R} \cup \text{MissExt}(\hat{R}, \hat{R}, I \cap I')$  which also respects the bound (17).

PROOF. Observe that  $L = (S' \cup \text{MissExt}(S', S', I')) \cap (S \cup \text{MissExt}(S, S, I))$ . First we will show that  $L \subseteq \hat{R} \cup \text{MissExt}(\hat{R}, \hat{R}, I \cap I')$ . Suppose  $w \in L$ . Then  $w$  belongs to at least one of the sets (1)  $S \cap S'$ , (2)  $S \cap \text{MissExt}(S', S', I')$ , (3)  $S' \cap \text{MissExt}(S, S, I)$ , or (4)  $\text{MissExt}(S, S, I) \cap \text{MissExt}(S', S', I')$ . We analyze each case:

- (1) Suppose  $w \in S \cap S'$ . If  $w \in \hat{R}$ , then clearly  $w \in \hat{R} \cup \text{MissExt}(\hat{R}, \hat{R}, I \cap I')$ . Suppose  $w \notin \hat{R}$ . Then there is word  $w' \in (O \cup O')^*$  and either a symbol  $\sigma \in O$  such that  $w \circ w' \circ \sigma \in S \setminus S'$  or a symbol  $\sigma \in O'$  such that  $w \circ w' \circ \sigma \in S' \setminus S$ . Write  $w = w_p \circ w''$  such that  $w''$  is the longest suffix of  $w$  which belongs to  $O \cup O'$ . It follows that the last symbol of  $w_p$  is an element of  $I \cap I'$ . Since  $w \notin \hat{R}$ , neither does  $w_p$ . This shows that for every word  $w_r \circ \sigma_r \in S \cap S'$  such that  $w_r \in \hat{R}$  but  $w_r \circ \sigma_r \notin \hat{R}$ , we must have  $\sigma_r \in I \cap I'$ .  
Let  $w'_p$  be the longest prefix of  $w_p$  which lies in  $\hat{R}$ . By assumption,  $\hat{R}$  is not empty. If we write  $w = w'_p \circ w''$ , the first symbol of  $w''$  is in  $I \cap I'$ . Thus,  $w \in \text{MissExt}(\hat{R}, \hat{R}, I \cap I')$ .
- (2) Observe that  $\text{MissExt}(S', S', I') = \text{MissExt}(S', S', I' \cap I) \cup \text{MissExt}(S', S', I' \cap O)$ . Moreover,  $S \cap \text{MissExt}(S', S', I \cap I') \subseteq \text{MissExt}(S \cap S', S \cap S', I \cap I') \subseteq \text{MissExt}(\hat{R}, \hat{R}, I \cap I')$ .  
Suppose  $w \in S \cap \text{MissExt}(S', S', I' \cap O)$ . Then  $w \in \text{Unc}(S', S, O, O')$ , so  $w \notin \hat{R}$ . Let  $w_i$  be the longest prefix of  $w$  which lies in  $S \cap S'$ . Then  $w_i \notin \hat{R}$ , either. Let  $w_p$  be the longest prefix of  $w_i$  which is in  $\hat{R}$ . Then  $w_i \in \text{MissExt}(\hat{R}, \hat{R}, I \cap I')$ , and therefore, so does  $w$ .
- (3) If  $w \in S' \cap \text{MissExt}(S, S, I)$ , an analogous reasoning applies.
- (4) Suppose  $w \in \text{MissExt}(S, S, I) \cap \text{MissExt}(S', S', I')$ . If  $w$  has a prefix in  $S' \cap \text{MissExt}(S, S, I)$  or  $S \cap \text{MissExt}(S', S', I')$ , then the reasoning of the last two points applies, and we have  $w \in \text{MissExt}(\hat{R}, \hat{R}, I \cap I')$ . Suppose  $w$  has no such a prefix, and write  $w = w_p \circ w'$ , where  $w_p$  is the longest prefix of  $w$  which lies in  $S \cap S'$ . Let  $\sigma$  be the first symbol of  $w'$ . Then  $w_p \circ \sigma \in \text{MissExt}(S, S, I) \cap \text{MissExt}(S', S', I')$ , which means that  $\sigma \in I \cap I'$ . Thus,  $w \in \text{MissExt}(S \cap S', S \cap S', I \cap I') \subseteq \text{MissExt}(\hat{R}, \hat{R}, I \cap I')$ .

We have shown that  $L \subseteq \hat{R} \cup \text{MissExt}(\hat{R}, \hat{R}, I \cap I')$ . Now suppose  $w \in \hat{R} \cup \text{MissExt}(\hat{R}, \hat{R}, I \cap I')$ . If  $w \in \hat{R}$  then clearly  $w \in S \cap S' \subseteq L$ . Suppose  $w \in \text{MissExt}(\hat{R}, \hat{R}, I \cap I')$  and let  $w_r$  be the longest prefix of  $w$  contained in  $\hat{R}$  and  $\sigma_r$  the symbol that comes immediately after  $w_r$  in  $w$ . Clearly  $\sigma_r \in I \cap I'$ .

If  $w_r \circ \sigma_r \in S \setminus S'$ , then  $w_r \circ \sigma_r$  cannot be an element of  $\hat{R}$ . If it were, we would have  $E_{\hat{R}} \times S \not\subseteq E_{S'}$ , violating the bound (17). The same applies when  $w_r \circ \sigma_r \in S' \setminus S$ .

If  $w_r \circ \sigma_r \notin S \cup S'$ , then  $w \circ \sigma_r \in \text{MissExt}(S', S', I') \cap \text{MissExt}(S, S, I) \subseteq L$ .

If  $w_r \circ \sigma_r \in S \cap S'$ , then  $w_r \circ \sigma_r \in \text{Unc}(S', S, O, O') \cup \text{Unc}(S, S', O', O)$ , which means that  $w_r \circ \sigma_r$  is not allowed to be an element of  $\hat{R}$ ; otherwise, there would be a contradiction of (17). ■

We conclude that  $R = \hat{R}$ . □
